# Supplementary material for: On the importance of hyperparameters in initializing parameterized quantum circuits
Source: arXiv:2604.21266 source file (2026-04-23)
Supplement: Supplementary file 1 [file table_qml.tex]

%%% Digits Beta Results %%%% 
\begin{tabular}{lrr}
\toprule
 & train_acc & test_acc \\
\midrule
score_beta_qfi & 0.879725 & 0.876712 \\
score_grad_beta & 0.865979 & 0.863014 \\
score_grad_beta_hybrid & 0.893471 & 0.835616 \\
manual & 0.896907 & 0.794521 \\
\bottomrule
\end{tabular}

%% Digits Gaussian Results %%% 
\begin{tabular}{lrr}
\toprule
 & train_acc & test_acc \\
\midrule
score_grad_gaussian_hybrid & 0.896907 & 0.794521 \\
score_grad_gaussian & 0.893471 & 0.794521 \\
score_gaussian_qfi & 0.879725 & 0.835616 \\
manual & 0.886598 & 0.794521 \\
\bottomrule
\end{tabular}

%%% Breast Cancer Beta Results %%%% 

\begin{tabular}{lrr}
\toprule
 & train_acc & test_acc \\
\midrule
score_grad_beta & 0.582418 & 0.561404 \\
score_beta_qfi & 0.602198 & 0.447368 \\
score_grad_beta_hybrid & 0.567033 & 0.605263 \\
manual & 0.573626 & 0.517544 \\
\bottomrule
\end{tabular}

%%% Breast Cancer Gaussian Results %%%% 

\begin{tabular}{lrr}
\toprule
 & train_acc & test_acc \\
\midrule
score_grad_gaussian & 0.571429 & 0.570175 \\
score_grad_gaussian_hybrid & 0.564835 & 0.622807 \\
score_gaussian_qfi & 0.575824 & 0.526316 \\
manual & 0.564835 & 0.596491 \\
\bottomrule
\end{tabular}

%%% Wine Beta Results %%%% 
\begin{tabular}{lrr}
\toprule
 & train_acc & test_acc \\
\midrule
score_grad_beta_hybrid & 0.971154 & 0.923077 \\
score_beta_qfi & 0.971154 & 0.961538 \\
score_grad_beta & 0.951923 & 0.961538 \\
manual & 0.971154 & 0.923077 \\
\bottomrule
\end{tabular}

%%% Wine Gaussian Results %%%% 

\begin{tabular}{lrr}
\toprule
 & train_acc & test_acc \\
\midrule
score_gaussian_qfi & 0.980769 & 0.884615 \\
score_grad_gaussian_hybrid & 0.971154 & 1.000000 \\
score_grad_gaussian & 0.971154 & 0.961538 \\
manual & 0.990385 & 0.807692 \\
\bottomrule
\end{tabular}
